# Supplementary material for: Abstracting Extensible Recursive Functions
Source: arXiv:2410.11742 source file (2025-07-21)
Supplement: Supplementary file 1 [file Appendix.tex]

\documentclass[rome.tex]{subfiles}

\usepackage{rome}

\begin{document}
\appendix

\section{Omitted Typing Rules}
\label{sec:extra-typing-rules}

\subsubsection*{Environment formation.}

\begin{small}
\begin{gather*}
\fbox{$\PEnvJ \Delta \Phi$} \; \; \fbox{$\TEnvJ \Delta \Gamma$}
\\
\begin{gathered}
\ib{\irule[\crule{pemp}]
          % {\KEnvJ \Delta};
          { };
          {\PEnvJ \Delta \varepsilon}}
\rsp
\ib{\irule[\crule{pvar}]
          {\PEnvJ \Delta \Phi}
          {\PredJ \Delta \pi};
          {\PEnvJ \Delta {\Phi, v : \pi}}}
\end{gathered}
\rsp
\begin{gathered}
\ib{\irule[\crule{temp}]
          %{\KEnvJ \Delta};
          { };
          {\TEnvJ \Delta \varepsilon}}
\rsp
\ib{\irule[\crule{tvar}]
          {\TEnvJ \Delta \Gamma}
          {\KindJ \Delta \tau \TypeK};
          {\TEnvJ \Delta {\Gamma, x : \tau}}}
\end{gathered}
\end{gather*}
\end{small}

\subsubsection*{Type equivalence.}

\begin{small}
\begin{gather*}
\fbox{$\TEqvJ \Delta \tau \tau \kappa$}
\\
\ib{\irule[\erule{refl}]
          {\KindJ \Delta \tau \kappa};
          {\TEqvJ \Delta \tau \tau \kappa}}
\rsp
\ib{\irule[\erule{sym}]
          {\TEqvJ \Delta {\tau_1} {\tau_2} \kappa};
          {\TEqvJ \Delta {\tau_2} {\tau_1} \kappa}}
\rsp
\ib{\irule[\erule{trans}]
          {\TEqvJ \Delta {\tau_1} {\tau_2} \kappa}
          {\TEqvJ \Delta {\tau_2} {\tau_3} \kappa};
          {\TEqvJ \Delta {\tau_1} {\tau_3} \kappa}}
\\
\ib{\irule[\erule{$\eta$}]
          {\KindJ \Delta {\phi} {\kappa_1 \to \kappa_2}};
          {\TEqvJ \Delta {\phi} {\lambda \alpha\co\kappa_1. \phi \, \alpha} {\kappa_1 \to \kappa_2}}}
\rsp
\ib{\irule[\erulec{\Sing {}}]
          {\TEqvJ \Delta {\xi_1} {\xi_2} \kappa};
          {\TEqvJ \Delta {\Sing{\xi_1}} {\Sing{\xi_2}} \TypeK}}
\rsp
\ib{\irule[\erulec {\then}]
          {\PEqvJ \Delta {\pi_1} {\pi_2}}
          {\TEqvJ \Delta {\tau_1} {\tau_2} \TypeK};
          {\TEqvJ \Delta {\pi_1 \then \tau_1} {\pi_2 \then \tau_2} \TypeK}}
\\
\ib{\irule[\erulec{\text{\textsc{app}}}]
          {\TEqvJ \Delta {\tau_1} {\upsilon_1} {\kappa \to \kappa'}}
          {\TEqvJ \Delta {\tau_2} {\upsilon_2} {\kappa}};
          {\TEqvJ \Delta {\tau_1\,\tau_2} {\upsilon_1\,\upsilon_2} {\kappa'}}}
\rsp
\ib{\irule[\esrule{$\xi_{\{\,\}}$}]
          {\TEqvJ \Delta {\xi\One_i} {\xi\Two_i} \LabK}
          {\TEqvJ \Delta {\tau\One_i} {\tau\Two_i} \kappa};
          {\TEqvJ \Delta {\RowIx i 1 n {\LabTy {\xi\One_i} {\tau\One_i}}} {\RowIx i 1 n {\LabTy {\xi\Two_i} {\tau\Two_i}}} {\RowK\kappa}}}
\\
\ib{\irule[\erulec {\forall}]
          {\TEqvJ {\Delta, \gamma\co\kappa} {\tau[\gamma/\alpha]} {\upsilon[\gamma/\beta]} \TypeK};
          {\TEqvJ \Delta {\forall\alpha\co\kappa.\tau} {\forall\beta\co\kappa.\upsilon} \TypeK}}
\rsp
\ib{\irule[\erulec {\lambda}]
          {\TEqvJ {\Delta, \gamma\co\kappa} {\tau[\gamma/\alpha]} {\upsilon[\gamma/\beta]} {\kappa'}};
          {\TEqvJ \Delta {\lambda\alpha\co\kappa.\tau} {\lambda\beta\co\kappa.\upsilon} {\kappa \to \kappa'}}}
\rsp
\text{($\gamma$ fresh for $\tau, \upsilon$)}
\\
\ib{\irule[\emrulec{\mu}]
          {\TEqvJ \Delta {\phi_1} {\phi_2} {\kappa \to \kappa}};
          {\TEqvJ \Delta {\RecTy {\phi_1}} {\RecTy {\phi_2}} \kappa}}
\rsp
\ib{\irule[\errulec{\Xi}]
          {\TEqvJ \Delta {\rho_1} {\rho_2} {\RowK\kappa}};
          {\TEqvJ \Delta {\Xi \rho_1} {\Xi \rho_2} {\kappa}}!
          {\Xi \in \Set {\Pi, \Sigma}}}
\\
\ib{\irule[\erulec{\lesssim}]
          {\TEqvJ \Delta {\tau_i} {\upsilon_i} {\RowK\kappa}};
          {\PEqvJ \Delta {\LeqP {\tau_1} {\tau_2}} {\LeqP {\upsilon_1} {\upsilon_2}}}}
\rsp
\ib{\irule[\erulec{\odot}]
          {\TEqvJ \Delta {\tau_i} {\upsilon_i} {\RowK\kappa}};
          {\PEqvJ \Delta {\PlusP {\tau_1} {\tau_2} {\tau_3}} {\PlusP {\upsilon_1} {\upsilon_2} {\upsilon_3}}}}
\end{gather*}
\end{small}

\section{Omitted data type definitions}
\label{sec:extra-data-types}

\subsubsection*{Unit}~
\begin{rosi}
type Unit : * 
type Unit = #'Unit 

tt : Unit
tt = #'Unit
\end{rosi}
\subsubsection*{Tuples}~
\begin{rosi}
type Pair : * -> * -> *
type Pair = \ t u. Pi {'1 := t, '2 := u}

pair : forall t u. t -> u -> Pair t u
pair = \x y. (#'1 := x) ++ (#'2 := y)

type Triple : * -> * -> * -> *
type Triple = \ t u v. Pi {'1 := t, '2 := u, '3 := v}

triple : forall t u v. t -> u -> v -> Triple t u v
triple = \x y z. pair x y ++ (#'3 := z)

fst = \x. sel x #'1
snd = \x. sel x #'2
thd = \x. sel x #'3
\end{rosi}

\subsubsection*{Naturals}~

\begin{rosi}
type NatF : * -> *
type NatF = \n. Sigma { 'Zero := Unit, 'Succ := n}

type Nat : *
type Nat = Mu NatF

zero : Nat
zero = in (inj (#'Zero := tt))

succ : Nat -> Nat
succ = \n. in (inj (#'Succ := n))

add : Nat -> Nat -> Nat
add = \m. fix (\add n. 
                 (case #'Zero (\u. m) 
               | case #'Succ (\nn. succ (add nn))) (out n))

one : Nat
one = succ zero

two : Nat
two = succ one

three : Nat
three = add one two
\end{rosi}

\subsubsection*{Lists}~
\begin{rosi}
type ListF : * -> * -> *
type ListF = \a. Sigma { 'Nil := Const Unit, 'Cons := (\l. Pair a l) }

type List : * -> *
type List = \a. Mu (ListF a)

nil : forall a. List a
nil = rcon #'Nil tt

cons : forall a. a -> List a -> List a
cons = \hd tl. rcon #'Cons (pair hd tl)

head : forall a. List a -> Maybe a
head = \l. match (out l)
           ( case #'Nil (const Nothing)
           | case #'Cons (o Just fst)
           )

tail : forall a. List a -> List a
tail = \l. match (out l)
           ( case #'Nil (const nil)
           | case #'Cons snd
           )

nth : forall a. List a -> Nat -> Maybe a
nth = fix (\f l n.
            match (out n)
            ( case #'Zero (const (head l))
            | case #'Succ (f (tail l))
            ))
\end{rosi}

\section{Omitted Code Samples}
\label{sec:extra-code-samples}

\subsubsection*{Evaluation: Boolean language}~

\begin{rosi}
type ValB : R[R[* -> *] -> * -> *]
type ValB = { 'Bool := (\ expr. \ val. Bool), 'Err := (\ expr. \ val. Unit) }
\end{rosi}
\codesep
\begin{rosi}
evalB : forall valr. ValB < valr =>
        Xh BoolF (\ expr. Env (valr expr) -> Mu (Sigma (valr expr)))
evalB = \ exp rec env.
           match exp
           ( case #'BConst (rcon #'Bool)
           | case #'If (\ t.
               as #'Bool (rec (sel t #'1) env)
               ( case #'True (const (rec (sel t #'2) env))
               | case #'False (const (rec (sel t #'3) env)))))
\end{rosi}

\section{Omitted Evaluation Definitions}
\label{sec:extra-evaluation}

\subsubsection*{The $pick$ function}

\begin{align*}
  \mathsf{pick} &: (\mathbb N \pto \mathbb N) \times (\mathbb N \pto \mathbb N) \times \mathbb N \pto \mathbb N + \mathbb N \\
  \mathsf{pick}(p, q, i) &= \begin{cases}
    \mathsf{Left} \, j &\text{if $p(j) = i$} \\
    \mathsf{Right} \, j &\text{if $q(j) = i$}
  \end{cases}
\end{align*}

\subsubsection*{The $dual$ function}

\[
\begin{aligned}
  \mathsf{dual} &: (\mathbb N \pto \mathbb N) \to \mathbb N \pto \mathbb N \\
  \mathsf{dual}(p, i) &= \mathsf{go}_p(i, 0)
\end{aligned}
\qquad\qquad
\begin{aligned}
  \mathsf{go}_p &: \mathbb N \pto \mathbb N \pto \mathbb N \\
  \mathsf{go}_p(0, j) &=
    \begin{cases}
      j &\text{if $j \not\in \ran(p)$} \\
      \mathsf{go}_p(0, j + 1) &\text{otherwise}
    \end{cases} \\
  \mathsf{go}_p(i, j) &=
    \begin{cases}
      \mathsf{go}_p(i, j + 1) &\text{if $j \in \ran(p)$} \\
      \mathsf{go}_p(i - 1, j + 1) &\text{otherwise}
    \end{cases}
\end{aligned}
\]

\end{document}
